# Supplementary material for: Off-Resonant Manipulation of Spins in Diamond via Precessing Magnetization of a Proximal Ferromagnet
Source: arXiv:1403.0656 source file (2014-03-04)
Supplement: Supplementary file 1 [file NVDiamondDynamicCouplingtoYIGSupplementary_Ver3.pdf]

# Supplementary Information: Off-Resonant Manipulation of Spins in Diamond via Precessing Magnetization of a Proximal Ferromagnet

C. S. Wolfe*,[1] V. P. Bhallamudi*,[1] H. L. Wang,[1] C. H. Du,[1] S. Manuilov,[1] A. J. Berger,[1] R. Adur,[1] F. Y. Yang,[1] and P. C. Hammel[1,*]

[1] *Department of Physics, The Ohio State University, Columbus, Ohio 43210, USA*

(Dated: February 27, 2014)

## I. FERROMAGNETIC RESONANCE

The ferromagnetic resonance (FMR) of the yttrium iron garnet (YIG) was measured by monitoring the reflected microwave power from our sample as we swept the magnetic field at a given microwave frequency and is plotted in Fig. S1 (a). A typical linecut of this data is shown in Fig. S1 (b), and we see a dip in the reflected power as the YIG undergoes resonance and absorbs power. By fitting the peak position vs. microwave frequency (Fig. S1 (c)) to the standard equation for the uniform mode FMR in this film and neglecting cubic anisotropy,[1]

$$\omega_0 = \gamma[B_0(B_0 + \mu_0 M)]^{1/2}$$

we obtain a saturation magnetization of 183 mT for our sample, as shown in Fig. S1 (c).

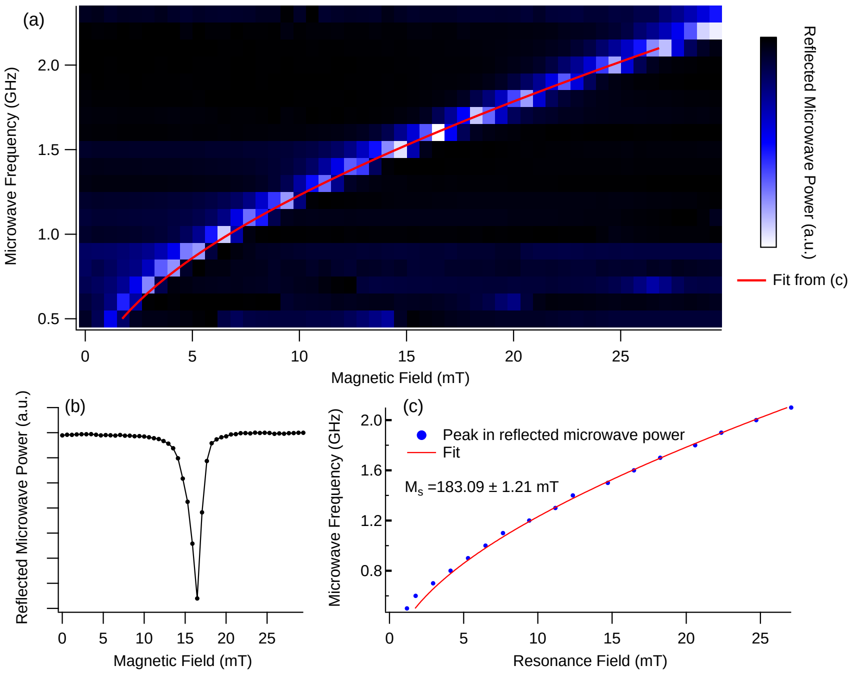


FIG. S1. **FMR data**: (a) Reflected microwave power measured as a function of magnetic field and microwave frequency. The microwaves were applied at approximately 30mW. Overlaid is the fit from (c). (b) A linecut of the data from (a) at a microwave frequency of 1.6 GHz. We see a dip when the YIG undergoes FMR. (c) The positions of the peaks in the microwave reflected power data are plotted vs. the microwave frequency and then fit to the equation for uniform mode FMR. From this we obtain $M_s = 183$ mT.

## II. THERMAL EFFECTS

The YIG film will absorb microwave power when it undergoes FMR, and this can result in heating of the nanodiamonds. The temperature dependence of NV center PL intensity in nanodiamonds has been reported to be $\sim 0.2\%/\mathrm{K}^2$. Here we will estimate the change in the PL that can result from the FMR heating. It is difficult to theoretically estimate the temperature change of the nanodiamonds, even with a known power absorption on FMR, due to uncertainties in estimating the thermal resistances at the various material interfaces. However, temperature change on FMR in YIG has been measured by An et.al.[?] and we will use their measurements to estimate the temperature change in our experiment. We will assume a worst case scenario, where the nanodiamond temperature tracks exactly the instantaneous YIG temperature.

Since we are measuring a lock-in signal, we are interesting in determining the temperature change on FMR during a half-cycle of our modulation period when the microwaves are on. The PL change due to this temperature change would approximately correspond to the lock-in signal we would measure due to FMR heating. We will assume that the change in temperature is related to the experimental parameters in the following manner:

$$\Delta T_{FMR} \propto E_{abs} \tag{S1}$$

$$\propto H_1^2 t\tau \tag{S2}$$

$$\propto \frac{P_{in}}{f} t\tau \tag{S3}$$

where, $\Delta T_{FMR}$ is the change of temperature due to the FMR, $E_{abs}$ is the energy absorbed per unit area, $H_1$ is the microwave magnetic field, $t$ the thickness of the YIG film, $\tau$ the time for which the microwaves are on, $P_{in}$ is the microwave power input to the sample, and $f$ is a factor that is related to the decrease in strength of $H_1$ due to the distance away from the microwave antenna.

Table 1 gives a comparison of our experimental parameters with those in An et.al[?] . Based on these values and their measured change of $\sim 10\,\mathrm{K/s}$ on FMR, we estimate temperature changes on FMR smaller than a $100\,\mu\mathrm{K}$ and changes in PL too small to be measured in our experiment.

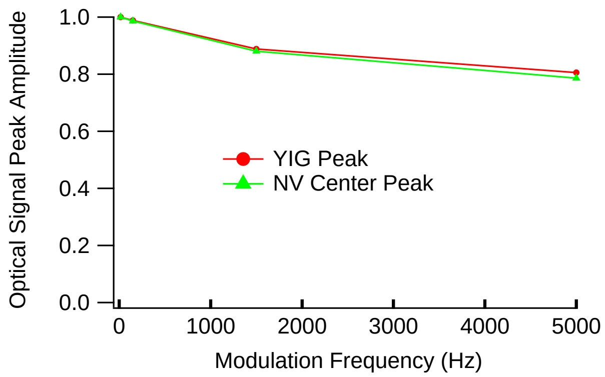


FIG. S2. **Thermal Effect Measurements**: Peaks in the optical signal, at the YIG FMR condition and the NV center resonance condition, are plotted vs. the frequency of the microwave amplitude modulation. These peaks are normalized to their values at 15 Hz. The red circles represent the amplitude of the peaks induced by the YIG FMR, and the green triangles represent the amplitude of the NV center resonance peaks. We attribute the drop in the signal with frequency to the response of our photdiode and preamplifier.

| Parameters | Our experiment | An et. al |
|---|---|---|
| $P_{in}$ (mW) | 35 | 230 |
| $f$ | 1 | 10 |
| $\nu$ (nm) | 20 | 30000 |
| $t$ (ms) | 3.5 | 1000 |

The result of the above analysis is consistent with our control experiments. First, we used Joule heating of the microwire to induce temperature changes in the nanodiamonds which were on GGG. The heating power was modulated between 0 and 3 mW at 150 Hz, the same frequency as was used for the data in Fig. 2 of the main text. Based on our reflected microwave power data, we expect the power absorbed on FMR to be more than 2 orders of magnitude smaller than 3 mW. The measured change in PL signal due to joule heating, even at 3 mW, is 2 orders smaller than the FMR-related peak seen our data in Fig. 2(c) of the main text.

Our second experiment was to measure the FMR-induced peak as a function of modulation frequency of the microwaves. We varied the modulation frequency from 15 Hz up to 5 kHz, the cut-off frequency of our preamplifier. Over this range the FMR-induced peak

behaves exactly same as the NV ground state peak (Fig. S2) and the slight reduction in amplitude with frequency is consistent with the specifications of the preamplifier. This data shows that if the effect is thermally driven, it has a time constant much faster than 5 KHz and will be inconsistent with the data in An. et.al.

Our analysis and the control experiments together show that heating does not play a significant part in our measured signal.

---

* hammel@physics.osu.edu

[2] T. Plakhotnik and D. Gruber, Phys. Chem. Chem. Phys. **12**, 9751 (2010).
